# Supplementary material for: Network analysis on cortical morphometry in first-episode schizophrenia
Source: arXiv:2212.13026 source file (2022-12-26)
Supplement: Supplementary file 1 [file Supplementary_materials.pdf]

**Table 1.**

Surface area (in mm) statistics of ROIs FES-vs-HC group differences after FWER correction. All 68 ROIs show no significant value in the test.

**Figure 1.**

Brain regions with significantly reduced clustering coefficient. The color bar reflects the p-value. Significant brain regions are colored dark blue and high-lighted with size (p<0.05).

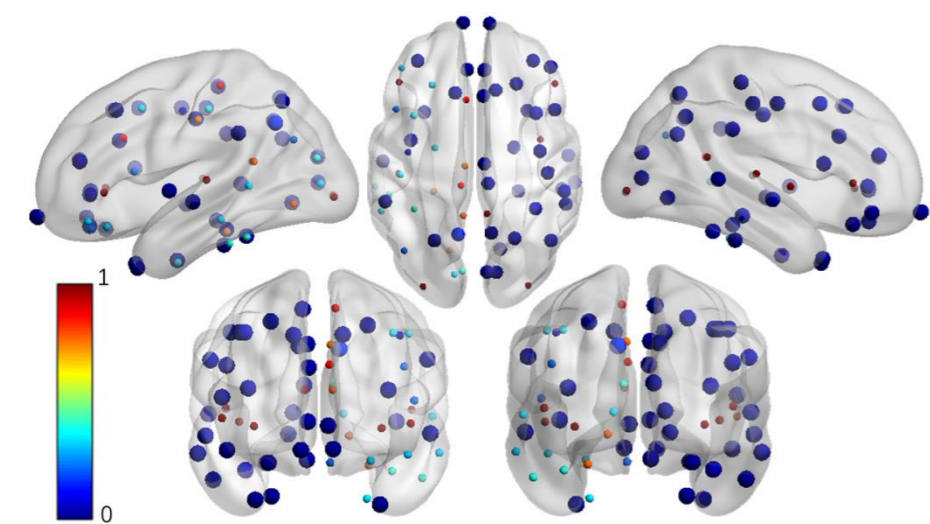

| ROIs                              | FES       | NC       | P-value | ROIs                               | FES      | NC       | P-value |
|-----------------------------------|-----------|----------|---------|------------------------------------|----------|----------|---------|
| bankssts (left)                   | 1044±196  | 1046±164 | 0.4703  | bankssts (right)                   | 764±146  | 798±149  | 0.0582  |
| caudal anterior cingulate (left)  | 676±170   | 672±143  | 0.4258  | caudal anterior cingulate (right)  | 630±185  | 600±148  | 0.1084  |
| caudal middle frontal (left)      | 2158±396  | 2194±311 | 0.2367  | caudal middle frontal (right)      | 2230±435 | 2180±390 | 0.1919  |
| cuneus (left)                     | 1576±296  | 1613±231 | 0.1532  | cuneus (right)                     | 1457±267 | 1476±205 | 0.2793  |
| entorhinal (left)                 | 422±100   | 425±105  | 0.4225  | entorhinal (right)                 | 393±94   | 385±77   | 0.2382  |
| fusiform (left)                   | 2969±414  | 3025±399 | 0.1748  | fusiform (right)                   | 2936±450 | 2984±408 | 0.2253  |
| inferior parietal (left)          | 4822±820  | 4969±721 | 0.0949  | inferior parietal (right)          | 5034±855 | 5051±757 | 0.4381  |
| inferior temporal (left)          | 3351±592  | 3493±497 | 0.0363  | inferior temporal (right)          | 3355±610 | 3445±537 | 0.1333  |
| isthmus cingulate (left)          | 993±197   | 997±169  | 0.4312  | isthmus cingulate (right)          | 963±201  | 956±149  | 0.3883  |
| lateral occipital (left)          | 5055±836  | 5038±646 | 0.4351  | lateral occipital (right)          | 4732±745 | 4839±606 | 0.1347  |
| lateral orbito frontal (left)     | 2603±386  | 2610±295 | 0.4342  | lateral orbito frontal (right)     | 2708±420 | 2781±374 | 0.1004  |
| lingual (left)                    | 2946±477  | 3040±442 | 0.0768  | lingual (right)                    | 3018±538 | 3071±498 | 0.2277  |
| medial orbito frontal (left)      | 1900±322  | 1883±255 | 0.3446  | medial orbito frontal (right)      | 1859±242 | 1865±200 | 0.4255  |
| middle temporal (left)            | 3269±531  | 3329±457 | 0.1954  | middle temporal (right)            | 3429±575 | 3527±494 | 0.1001  |
| parahippocampal (left)            | 609±91    | 618±76   | 0.2136  | para hippocampal (right)           | 663±104  | 680±97   | 0.1199  |
| paracentral (left)                | 1271±189  | 1298±170 | 0.1507  | para central (right)               | 1492±232 | 1499±192 | 0.4169  |
| pars opercularis (left)           | 1599±287  | 1604±276 | 0.4523  | pars opercularis (right)           | 1361±262 | 1364±212 | 0.4835  |
| pars orbitalis (left)             | 655±125   | 657±95   | 0.4404  | pars orbitalis (right)             | 805±137  | 816±124  | 0.2728  |
| pars triangularis (left)          | 1327±262  | 1323±243 | 0.4513  | pars triangularis (right)          | 1526±321 | 1536±292 | 0.4033  |
| pericalcarine (left)              | 1449±305  | 1515±270 | 0.0533  | pericalcarine (right)              | 1481±317 | 1530±282 | 0.1219  |
| postcentral (left)                | 3838±624  | 3913±504 | 0.1712  | postcentral (right)                | 4144±668 | 4192±544 | 0.2901  |
| posterior cingulate (left)        | 1256±270  | 1250±219 | 0.4284  | posterior cingulate (right)        | 1146±192 | 1136±174 | 0.3438  |
| precentral (left)                 | 4741±696  | 4840±586 | 0.1414  | precentral (right)                 | 4769±704 | 4769±549 | 0.4995  |
| precuneus (left)                  | 3864±566  | 3901±495 | 0.3201  | precuneus (right)                  | 3913±603 | 3948±525 | 0.3339  |
| rostral anterior cingulate (left) | 750±173   | 762±150  | 0.2954  | rostral anterior cingulate (right) | 641±181  | 627±137  | 0.2753  |
| rostral middle frontal (left)     | 5950±1044 | 5977±876 | 0.4173  | rostral middle frontal (right)     | 5744±993 | 5865±882 | 0.1797  |
| superior frontal (left)           | 7126±967  | 7128±814 | 0.4940  | superior frontal (right)           | 6759±945 | 6822±770 | 0.3065  |
| superior parietal (left)          | 5303±842  | 5440±729 | 0.1107  | superior parietal (right)          | 5171±780 | 5205±683 | 0.3751  |
| superior temporal (left)          | 3782±567  | 3804±447 | 0.3772  | superior temporal (right)          | 3629±546 | 3731±507 | 0.0906  |
| supramarginal (left)              | 3641±647  | 3675±655 | 0.3538  | supramarginal (right)              | 3991±720 | 4047±633 | 0.2865  |
| frontal pole (left)               | 263±37    | 256±32   | 0.0766  | frontal pole (right)               | 296±33   | 295±31   | 0.4045  |
| temporal pole (left)              | 463±70    | 456±65   | 0.2317  | temporal pole (right)              | 482±68   | 475±67   | 0.2311  |
| transverse temporal (left)        | 418±70    | 427±59   | 0.1529  | transverse temporal (right)        | 347±65   | 360±54   | 0.0568  |
| insula (left)                     | 2495±388  | 2472±352 | 0.324   | insula (right)                     | 2375±376 | 2366±285 | 0.4315  |

**Table 2.**

The cortical thickness network parameters and corresponding p-values calculated by FES-vs-HC group comparisons via permutation test at different densities.

The thresholds are set from 0.1101 to 0.5 with a 0.02 step size.

| Threshold= | $\gamma$     | $\lambda$ | $\sigma$     | C            | L     | T            | B_edge | B_nodal | Q     | E_global | E_local      | r     |
|------------|--------------|-----------|--------------|--------------|-------|--------------|--------|---------|-------|----------|--------------|-------|
| 0.1102     | <b>0.032</b> | 0.501     | <b>0.032</b> | <b>0.034</b> | 0.259 | <b>0.027</b> | 0.263  | 0.240   | 0.386 | 0.671    | <b>0.033</b> | 0.321 |
| 0.1299     | 0.200        | 0.471     | 0.196        | 0.200        | 0.712 | 0.147        | 0.543  | 0.629   | 0.858 | 0.370    | 0.155        | 0.274 |
| 0.1501     | 0.478        | 0.411     | 0.473        | 0.514        | 0.924 | 0.323        | 0.646  | 0.749   | 0.734 | 0.357    | 0.50         | 0.259 |
| 0.1699     | 0.200        | 0.421     | 0.198        | 0.209        | 0.664 | 0.211        | 0.716  | 0.869   | 0.690 | 0.349    | 0.143        | 0.264 |
| 0.1901     | 0.406        | 0.477     | 0.378        | 0.387        | 0.995 | 0.358        | 0.723  | 0.900   | 0.496 | 0.37     | 0.186        | 0.266 |
| 0.2098     | 0.795        | 0.516     | 0.752        | 0.640        | 0.907 | 0.400        | 0.731  | 0.968   | 0.681 | 0.386    | 0.263        | 0.438 |
| 0.2300     | 0.925        | 0.409     | 0.92         | 0.792        | 0.964 | 0.506        | 0.827  | 0.853   | 0.709 | 0.339    | 0.440        | 0.282 |
| 0.2502     | 0.936        | 0.411     | 0.939        | 0.940        | 0.586 | 0.702        | 0.822  | 0.819   | 0.469 | 0.348    | 0.852        | 0.296 |
| 0.2700     | 0.875        | 0.393     | 0.869        | 0.973        | 0.933 | 0.816        | 0.865  | 0.694   | 0.904 | 0.317    | 0.969        | 0.289 |
| 0.2902     | 0.731        | 0.435     | 0.734        | 0.879        | 0.681 | 0.936        | 0.833  | 0.691   | 0.942 | 0.324    | 0.704        | 0.434 |
| 0.3099     | 0.637        | 0.41      | 0.635        | 0.748        | 0.859 | 0.913        | 0.832  | 0.677   | 0.747 | 0.295    | 0.529        | 0.339 |
| 0.3301     | 0.604        | 0.439     | 0.604        | 0.694        | 0.926 | 0.841        | 0.797  | 0.793   | 0.665 | 0.316    | 0.496        | 0.536 |
| 0.3499     | 0.555        | 0.419     | 0.555        | 0.642        | 0.759 | 0.741        | 0.801  | 0.877   | 0.871 | 0.330    | 0.457        | 0.979 |
| 0.3701     | 0.599        | 0.359     | 0.598        | 0.674        | 0.826 | 0.747        | 0.741  | 0.821   | 0.204 | 0.356    | 0.457        | 0.784 |
| 0.3898     | 0.503        | 0.490     | 0.503        | 0.564        | 0.738 | 0.636        | 0.809  | 0.854   | 0.713 | 0.427    | 0.425        | 0.930 |
| 0.4100     | 0.516        | 0.654     | 0.516        | 0.552        | 0.985 | 0.609        | 0.649  | 0.904   | 0.908 | 0.594    | 0.409        | 0.764 |
| 0.4302     | 0.502        | 0.801     | 0.502        | 0.554        | 0.431 | 0.610        | 0.834  | 0.554   | 0.730 | 0.742    | 0.412        | 0.767 |
| 0.4500     | 0.496        | 0.884     | 0.496        | 0.535        | 0.782 | 0.589        | 0.986  | 0.199   | 0.693 | 0.855    | 0.408        | 0.734 |
| 0.4701     | 0.445        | 0.947     | 0.445        | 0.477        | 0.903 | 0.528        | 0.916  | 0.634   | 0.962 | 0.916    | 0.370        | 0.760 |
| 0.4899     | 0.439        | 0.974     | 0.439        | 0.460        | 0.532 | 0.492        | 0.685  | 0.834   | 0.157 | 0.948    | 0.369        | 0.696 |

**Table 3.**

The cortical thickness network parameters and corresponding p-values calculated by FES-vs-HC group comparisons via permutation test at different densities.

The thresholds are set from 0.1400 to 0.5 with a 0.02 step size.

| Threshold= | $\gamma$ | $\lambda$ | $\sigma$ | C     | L     | T            | B_edge | B_nodal | Q     | E_global | E_local | r     |
|------------|----------|-----------|----------|-------|-------|--------------|--------|---------|-------|----------|---------|-------|
| 0.1400     | 0.079    | 0.430     | 0.078    | 0.997 | 0.769 | <b>0.048</b> | 0.144  | 0.122   | 0.069 | 0.928    | 0.327   | 0.578 |
| 0.1600     | 0.161    | 0.471     | 0.387    | 0.995 | 0.68  | 0.057        | 0.732  | 0.872   | 0.360 | 0.913    | 0.317   | 0.556 |
| 0.1800     | 0.284    | 0.494     | 0.402    | 0.897 | 0.711 | 0.097        | 0.722  | 0.900   | 0.555 | 0.751    | 0.331   | 0.920 |
| 0.2000     | 0.381    | 0.410     | 0.389    | 0.755 | 0.587 | 0.072        | 0.813  | 0.905   | 0.592 | 0.522    | 0.287   | 0.769 |
| 0.2200     | 0.515    | 0.396     | 0.522    | 0.785 | 0.536 | 0.072        | 0.866  | 0.773   | 0.615 | 0.514    | 0.273   | 0.709 |
| 0.2400     | 0.413    | 0.429     | 0.42     | 0.654 | 0.565 | 0.043        | 0.857  | 0.777   | 0.761 | 0.417    | 0.301   | 0.917 |
| 0.2600     | 0.399    | 0.472     | 0.413    | 0.605 | 0.585 | 0.120        | 0.837  | 0.763   | 0.984 | 0.412    | 0.318   | 0.819 |
| 0.2800     | 0.397    | 0.401     | 0.396    | 0.572 | 0.511 | 0.212        | 0.875  | 0.644   | 0.629 | 0.378    | 0.277   | 0.631 |
| 0.3000     | 0.434    | 0.464     | 0.436    | 0.544 | 0.565 | 0.249        | 0.805  | 0.73    | 0.574 | 0.397    | 0.326   | 0.585 |
| 0.3200     | 0.464    | 0.511     | 0.465    | 0.56  | 0.634 | 0.305        | 0.748  | 0.825   | 0.811 | 0.491    | 0.368   | 0.927 |
| 0.3400     | 0.437    | 0.484     | 0.44     | 0.495 | 0.692 | 0.408        | 0.708  | 0.942   | 0.40  | 0.453    | 0.407   | 0.866 |
| 0.3600     | 0.461    | 0.463     | 0.465    | 0.523 | 0.884 | 0.394        | 0.729  | 0.738   | 0.609 | 0.454    | 0.403   | 0.705 |
| 0.3800     | 0.424    | 0.426     | 0.424    | 0.454 | 0.872 | 0.46         | 0.690  | 0.792   | 0.417 | 0.437    | 0.408   | 0.732 |
| 0.4000     | 0.404    | 0.557     | 0.403    | 0.411 | 0.914 | 0.521        | 0.853  | 0.764   | 0.119 | 0.389    | 0.530   | 0.945 |
| 0.4200     | 0.379    | 0.715     | 0.38     | 0.410 | 0.962 | 0.543        | 0.716  | 0.507   | 0.543 | 0.361    | 0.685   | 0.872 |
| 0.4400     | 0.423    | 0.844     | 0.423    | 0.447 | 0.985 | 0.512        | 0.497  | 0.533   | 0.817 | 0.386    | 0.813   | 0.842 |
| 0.4600     | 0.457    | 0.919     | 0.457    | 0.479 | 0.992 | 0.491        | 0.418  | 0.838   | 0.913 | 0.392    | 0.897   | 0.667 |
| 0.4800     | 0.428    | 0.955     | 0.428    | 0.464 | 0.994 | 0.489        | 0.792  | 0.813   | 0.565 | 0.376    | 0.939   | 0.508 |
| 0.5000     | 0.450    | 0.989     | 0.450    | 0.46- | 0.998 | 0.491        | 0.563  | 0.623   | 0.437 | 0.367    | 0.960   | 0.613 |

**Table 4.**

The brain regions show that some have achieved statistical significance in FES-vs-HC group comparisons via 1-tailed permutation test ( $p < 0.05$ ).

| ROIs                               | clustering coefficient |    |         | Local efficiency |    |         |
|------------------------------------|------------------------|----|---------|------------------|----|---------|
|                                    | FES                    | HC | P-value | FES              | HC | P-value |
| precuneus(left)                    | 0                      | 0  | 0.014   | 0                | 0  | 0.014   |
| Rostral anterior cingulate(left)   | 0                      | 0  | 0.002   | 0                | 0  | 0.002   |
| Rostral middle frontal (left)      | 0                      | 0  | 0.001   | 0                | 0  | 0.001   |
| Superior frontal(left)             | 0                      | 0  | 0.002   | 0                | 0  | 0.002   |
| Superior parietal(left)            | 0                      | 0  | 0.001   | 0                | 0  | 0.001   |
| superiortemporal(left)             | 0                      | 0  | 0.001   | 0                | 0  | 0.001   |
| supramarginal(left)                | 0                      | 0  | 0.001   | 0                | 0  | 0.001   |
| Frontal pole(left)                 | 0                      | 0  | 0.001   | 0                | 0  | 0.001   |
| temporalpole(left)                 | 0                      | 0  | <e-4    | 0                | 0  | <e-4    |
| insula(left)                       | 0                      | 0  | <e-4    | 0                | 0  | <e-4    |
| bankssts(right)                    | 0                      | 0  | <e-4    | 0                | 0  | <e-4    |
| caudalanteriorcingulate(right)     | 0                      | 0  | 0.001   | 0                | 0  | 0.001   |
| caudalmiddlefrontal(right)         | 0                      | 0  | 0.004   | 0                | 0  | 0.004   |
| cuneus(right)                      | 0                      | 0  | 0.001   | 0                | 0  | 0.001   |
| entorhinal(right)                  | 0                      | 0  | <e-4    | 0                | 0  | <e-4    |
| fusiform(right)                    | 0                      | 0  | 0.004   | 0                | 0  | 0.004   |
| inferiorparietal(right)            | 0                      | 0  | 0.001   | 0                | 0  | 0.001   |
| inferiortemporal(right)            | 0                      | 0  | <e-4    | 0                | 0  | <e-4    |
| lateralorbitofrontal(right)        | 24.659                 | 0  | <e-4    | 24.659           | 0  | <e-4    |
| lingual(right)                     | 0                      | 0  | <e-4    | 0                | 0  | <e-4    |
| medialorbitofrontal(right)         | 0                      | 0  | 0.001   | 0                | 0  | 0.001   |
| Middle temporal(right)             | 0                      | 0  | 0.001   | 0                | 0  | 0.001   |
| parahippocampal(right)             | 10.462                 | 0  | 0.002   | 10.462           | 0  | 0.002   |
| paracentral(right)                 | 0                      | 0  | 0.001   | 0                | 0  | 0.001   |
| parsopercularis(right)             | 0                      | 0  | <e-4    | 0                | 0  | <e-4    |
| Pars orbitalis(right)              | 0                      | 0  | 0.002   | 0                | 0  | 0.002   |
| pericalcarine(right)               | 0                      | 0  | <e-4    | 0                | 0  | <e-4    |
| postcentral(right)                 | 0                      | 0  | 0.004   | 0                | 0  | 0.004   |
| Posterior cingulate(right)         | 0                      | 0  | 0.001   | 0                | 0  | 0.001   |
| precentral(right)                  | 0                      | 0  | 0.003   | 0                | 0  | 0.003   |
| precuneus(right)                   | 0                      | 0  | <e-4    | 0                | 0  | <e-4    |
| Rostral anterior cingulate (right) | 0                      | 0  | 0.001   | 0                | 0  | 0.001   |
| Rostral middle frontal (right)     | 0                      | 0  | 0.002   | 0                | 0  | 0.002   |
| Superior frontal (right)           | 0                      | 0  | 0.001   | 0                | 0  | 0.001   |
| Superior parietal (right)          | 0                      | 0  | 0.001   | 0                | 0  | 0.001   |
| Superior temporal (right)          | 0                      | 0  | 0.002   | 0                | 0  | 0.002   |
| Supramarginal (right)              | 0                      | 0  | 0.003   | 0                | 0  | 0.003   |
| Frontal pole (right)               | 32.879                 | 0  | <e-4    | 32.879           | 0  | <e-4    |
| Temporal pole (right)              | 0                      | 0  | 0.002   | 0                | 0  | 0.002   |
